# Supplementary material for: Optimizing for ROC Curves on Class-Imbalanced Data by Training over a Family of Loss Functions
Source: arXiv:2402.05400 source file (2024-06-04)
Supplement: Supplementary file 1 [file appendix_related_work.tex]

\section{Detailed related work}
\label{sec:appendix_related}

Training on imbalanced datasets with algorithms designed to work on balanced datasets can be problematic because the gradients and losses are biased towards the common classes, so the rare classes will not be learned well. Current methods to mitigate the effects of training under imbalance include methods that modify the loss functions, re-sample and augment training samples, and improve the module via two-stage learning, ensembles, or representation learning \cite{zhang2023deep}. 

\subsection{Specialized loss functions}
% Other types of loss adjustments
To balance the gradients from all classes, several papers adaptively change a sample's weight in the loss based on features such as the sample's confidence score, class frequency, and influence on model weights \cite{zhang2021distribution, fernando2021dynamically, park2021influence, wang2021seesaw, li2021autobalance}.
Other work addresses the difference in the norms of features associated with frequent (head) and rare (tail) classes and proposes to balance this by utilizing a feature-based loss~\cite{li2022feature} or weight-decay and gradient clipping~\cite{alshammari2022long}.

% Loss functions closely related to VS loss
Some work has focused on enforcing larger margins on the tail classes using additive factors on the logits in Cross-entropy loss \cite{cao2019learning, menon2021longtail, li2022long}. Other work proposed adding multiplicative factors to the logits to adjust for the difference in the magnitude of minority-class logits at training and test time or minimize a margin-based generalization bound \cite{Ye2020-yj, kang2021learning}. \citet{kini2021labelimbalanced} show that multiplicative factors are essential for the terminal phase of training, but that these have negative effects early during training, so additive factors are necessary to speed up convergence. They propose Vector Scaling (VS) loss as a general loss function that includes both additive and multiplicative factors on the logits. \citet{behnia2023implicit} study the implicit geometry of classifiers trained on a special case of VS loss. 

% Imbalance in CV applications
Beyond classification, many papers have focused on imbalance in instance segmentation and object detection applications~\cite{tan2021equalization, wang2021adaptive, feng2021exploring, li2020overcoming}. ~\citet{ren2022balanced} also propose a balanced Mean Square Error (MSE) loss for regression problems, such as age and depth estimation.

\subsection{Data-level methods}
Another way to balance the gradients of classes during training is resampling. This could be done by sampling the minority class more often (random over-sampling) or sampling the majority class less often (random under-sampling) \cite{Johnson2019-xu, Japkowicz00theclass, Liu2009-rs}. \citet{jiang2023semi, hou2023subclass} use clustering to drive resampling; specifically, they cluster head classes into multiple clusters and then resample across clusters instead of classes. Meta-learning has been used to estimate the optimal sampling rates of different classes~\cite{ren2020balanced}, while \citet{wang2019dynamic} dynamically adapts both the loss function and sampling procedure throughout training.

Additionally, data augmentation can be used alongside oversampling to increase the size of the minority class samples and enable model generalization~\cite{zhong2021improving, zang2021fasa, li2021metasaug, du2023global}. With tabular data, small perturbations of random noise can be added to generate new examples. Images lend themselves to more high-level augmentations. Methods that copy and paste patches of images, such as CutMix~\cite{yun2019cutmix} and PuzzleMix~\cite{kim2020puzzle} have been used to improve classification or instance segmentation~\cite{Ghiasi2020-ei} performance.

SMOTE (Synthetic Minority Over-sampling Technique) creates synthetic examples by interpolating between samples in the same class of the training set \cite{Chawla2011-eb}. The interpolation is done in feature space instead of data space. 
The mixup method also generates synthetic examples; however, unlike SMOTE, it interpolates between samples of different classes \cite{zhang2018mixup}. These synthetic examples are given a soft label that corresponds to the proportion of input from each class. StyleMix adapts mixup to separately manipulate an image's content and style~\cite{Hong2021-ex}. ReMix advances mixup to optimize for situations with class imbalance by combining mixup and resampling \cite{Bellinger2020-om}. \citet{li2021metasaug} creates augmented data samples by translating deep features along semantically meaningful directions. \citet{zada2022pure} adds pure noise images to the training set and introduces a new type of distribution-aware batch normalization layer to facilitate training with them.

\subsection{Module improvements}
% Contrastive learning
Some work has shown that overly emphasizing the minority class can disrupt the original data distribution and cause overfitting~\cite{zhou2020bbn, du2023global} or reduce the accuracy of the majority class~\cite{zhu2022balanced}. To mitigate this issue, contrastive learning~\cite{du2023global, zhu2022balanced, wang2021contrastive} has been used to learn a robust feature representation by enforcing consistency between two differently augmented versions of the data. \citet{du2023global} devise a single-stage approach, by combining the ideas of contrastive representations with soft label class re-weighting to achieve state-of-the-art performance on several benchmarks. 

% Features and multi-expert
Multi-expert methods have also been explored~\cite{zhang2022self, wang2020long, li2022nested}. ~\citet{li2022nested} collaboratively learn multiple experts, by learning individual experts and transferring knowledge among them, in a nested way. Methods have also used two branches or heads with one classification branch along with another branch, either to re-balance~\cite{guo2021long, zhou2020bbn} or calibrate~\cite{wang2020devil} the model. \citet{tang2022invariant} adopt a generalized approach to learn attribute-invariant features that first discovers sets of samples with diverse intra-class distributions from the low confidence predictions, and then learns invariant features across them. \citet{dong2022lpt} uses language prompts to improve both general and group-specific features.
